# Supplementary material for: Characterizing State Space Model and Hybrid Language Model Performance with Long Context
Source: arXiv:2507.12442 source file (2026-03-22)
Supplement: Supplementary file 1 [file 09_Appendix_A.tex]

\clearpage
\appendices
\section*{Artifact Appendix}
%%%%%%%%%%%%%%%%%%%%%%%%%%%%%%%%%%%%%%%%%%%%%%%%%%%%%%%%%%%%%%%%%%%%%
\subsection{Abstract}
This appendix describes the workflow to run \bench and reproduce the results reported in the paper. 


\subsection{Artifact check-list (meta-information)}

{\small
\begin{itemize}
  \item {\textbf{Algorithm}: Profiling functions are deployment flow specific. We use the PyTorch Profiler~\cite{pytorch_profiler} for PyTorch, EP Profiling for ONNX RUNTIME~\cite{onnxruntime}, and TensorRT Open Source Software (OSS) for TensorRT~\cite{trt_oss}. }
  % 
  \item {\textbf {Program}: Python 3.10, CUDA 12.6.}
  % 
  \item {\textbf{Model:} Please refer to~\autoref{tab:modeltable}.}
  % 
  \item {\textbf {Data set:} Please refer to~\autoref{tab:modeltable}. }
  % 
  \item {\textbf {Run-time environment:} Tested Environments: Ubuntu 22.04, Linux Mint 21.1, and MacOS 14.2.1.}
  % 
  \item {\textbf {Hardware:} AMD EPYC 7763 CPU, 1TB DDR4 RAM, 1 x NVIDIA A100 80GB (PCIe), Intel i9-13900K, 64 GB DDR5 RAM, and Nvidia RTX 4090 24GB (PCIe).  }
  % 
  \item {\textbf {Execution:} Automated Scripts. Please refer to the README file in the Github repository. }
  \item {\textbf {Metrics:} Latency.}
  % 
  \item {\textbf {Output:} Plots in PNG format, and the corresponding data in csv format. The automated scripts plot the operator level end-to-end inference latency breakdown of all \bench profiled models.}
  % 
  \item {\textbf {Experiments:} Please refer to \autoref{sec:case_studies} for more details.  }
  % 
  \item {\textbf {How much disk space required (approximately)?:} Approximately 100 GB to store the models, the datasets, and the collected profiling traces.}
  % 
  \item {\textbf {How much time is needed to prepare workflow (approximately)?:} Approximately, setting up the workflow requires around 30 minutes. }
  % 
  \item {\textbf {How much time is needed to complete experiments (approximately)?:} Approximately 10 hours.}
  \item {\textbf {Publicly available?:} https://doi.org/10.5281/zenodo.15043135}
  \item {\textbf {Code licenses (if publicly available)?:}  MIT License. }
  \item {\textbf {Archived (provide DOI)?:} 10.5281/zenodo.15043135 }
\end{itemize}
}

%%%%%%%%%%%%%%%%%%%%%%%%%%%%%%%%%%%%%%%%%%%%%%%%%%%%%%%%%%%%%%%%%%%%%
\subsection{Description}

\subsubsection{How to access}
The source code is available on Zenodo at   https://doi.org/10.5281/zenodo.15043135, or on Github at https://github.com/UCI-ISA-Lab/NonGEMM-Bench-ISPASS25.git. 

\subsubsection{Hardware dependencies}
To reproduce the paper's results, the following systems are required: 
\begin{itemize}
% 
\item{Server with an AMD EPYC 7763 CPU, 1TB DDR4 RAM, 1x Nvidia A100 80GB GPU. (We note that the Mixture of Experts model profiling requires 4x Nvidia A100 80GB GPUs.) }
% 
\item{Workstation with an Intel i9-13900K, 64 GB DDR5 RAM, 1x Nvidia RTX 4090 24 GB GPU.}
\end{itemize}
Nevertheless, our workflow runs on any typical laptop, workstation, or server system with a CUDA-capable GPU. 

\subsubsection{Software dependencies}
\begin{itemize}
\item{Python 3.10}
% 
\item{CUDA 12.6}
% 
\item{TensorRT 10.4.0.26}
% 
\item{TensorRT Open Source Software}
% 
\item{PyTorch}
% 
\item{Torchvision}
% 
\item{ONNX Runtime}
% 
\item{Hugging Face Transformers}
% 
\item{Hugging Face Datasets}
% 
\item{Hugging Face Optimum}
% 
\item{Hugging Face Accelerate}
% 
\item{Matplotlib}
% 
\item{COCO API}
% 
\item{Access to Llama 2 Weights on Hugging Face}
% 
\item{Access to Llama 3 Weights on Hugging Face}
\item{Access to Mixtral 8x7B Weights on Hugging Face}
\end{itemize}

\subsubsection{Data sets}
We use three publicly available datasets highlighted in~\autoref{tab:modeltable}: ImageNet~\cite{imagenet_cvpr09}, COCO~\cite{lin2014microsoft}, and wikitext~\cite{wikitext}

\subsubsection{Models}
We use 17 popular pretrained models from Huggingface and Torchvision. Please refer to~\autoref{tab:modeltable} for the detailed list.

%%%%%%%%%%%%%%%%%%%%%%%%%%%%%%%%%%%%%%%%%%%%%%%%%%%%%%%%%%%%%%%%%%%%%
\subsection{Installation}
\subsubsection {PyTorch and ONNX Runtime Flow Software Dependency Installation}
% 


\begin{verbatim}
> cd torch_flow
> conda create -n ng-torch python=3.10
> pip install -r requirements.txt 
> ## After setting up the conda environment, 
> ## Install the COCO dataset dependencies.
\end{verbatim}
Please refer to the code base for more details. 

\subsubsection{TensorRT Flow Software Dependency Installation}

\begin{verbatim}
> cd trt_flow
> conda create -n ng-trt python=3.10
> pip install -r requirements.txt 
\end{verbatim}
After setting up the conda environment, please refer to the TensorRT OSS Github repository (https://github.com/NVIDIA/TensorRT/tree/release/10.4) to setup TensorRT. 

%%%%%%%%%%%%%%%%%%%%%%%%%%%%%%%%%%%%%%%%%%%%%%%%%%%%%%%%%%%%%%%%%%%%%
\subsection{Experiment workflow}
\begin{verbatim}
> cd torch_flow
> conda activate ng-torch
> ## Set the path to ImageNet and COCO datasets in run.py
> bash run_ispass_all.sh
> cd ../onnx_flow 
> bash run_ispass_all.sh
> cd ../trt_flow 
> conda activate ng-trt
> ## Set the path to your TensorRT OSS
> ## installation in setup.sh
> bash run_ispass_all.sh

\end{verbatim}

\textbf{Note:} Before running the experiments, environment variables and global constants should be properly set to configure the path to the datasets and to the TensorRT tools. Please refer to the README file in the codebase.
%%%%%%%%%%%%%%%%%%%%%%%%%%%%%%%%%%%%%%%%%%%%%%%%%%%%%%%%%%%%%%%%%%%%%
\subsection{Evaluation and expected results}

Running the \texttt{run\_ispass\_all.sh} scripts in every subdirectory will reproduce~\autoref{fig:server_op_breakdown_camera_ready}, ~\autoref{fig:llm_onnx_vs_eager_camera-ready} , ~\autoref{fig:server_trt_cv_inductor_camera_ready}, and ~\autoref{fig:server_quantization_camera_ready}. 

The scripts will generate the plots and the corresponding CSV data in the \texttt{torch\_flow/summary}, \texttt{onnx\_flow/fig6\_onnx}, and \texttt{trt\_flow/fig7\_trt}. The raw data is stored in \texttt{non-gemm-out} directory. 
% 
The reproduced latency results are expected to be close to the results in the paper, but not an exact match because of potential differences in the hardware or software environment. 
% 



%%%%%%%%%%%%%%%%%%%%%%%%%%%%%%%%%%%%%%%%%%%%%%%%%%%%%%%%%%%%%%%%%%%%%
\subsection{Experiment customization}
The provided scripts run the entire evaluation presented in the paper. 
%  
The users can customize their experiments by modifying the following files: 
\begin{itemize}
\item{\textbf{Modifying datasets and profiling settings:} Please modify corresponding variables in \texttt{torch\_flow/run.py}.}
% 
\item{\textbf{Profiling new models:} Please refer to \texttt{ModelProfile} class in \texttt{torch\_flow/run.py} and add the desired model to the file.}

\end{itemize}

%%%%%%%%%%%%%%%%%%%%%%%%%%%%%%%%%%%%%%%%%%%%%%%%%%%%%%%%%%%%%%%%%%%%%
\subsection{Methodology}

Submission, reviewing and badging methodology:

\begin{itemize}
  \item \url{https://www.acm.org/publications/policies/artifact-review-and-badging-current}
  \item \url{https://cTuning.org/ae}
\end{itemize}
